# Supplementary material for: MeTTA: Single-View to 3D Textured Mesh Reconstruction with Test-Time Adaptation
Source: arXiv:2408.11465 source file (2024-08-21)
Supplement: Supplementary file 2 [file radius_abla.tex]

\begin{figure}[h]
  \small
  \centering
    \includegraphics[width=0.9\linewidth]{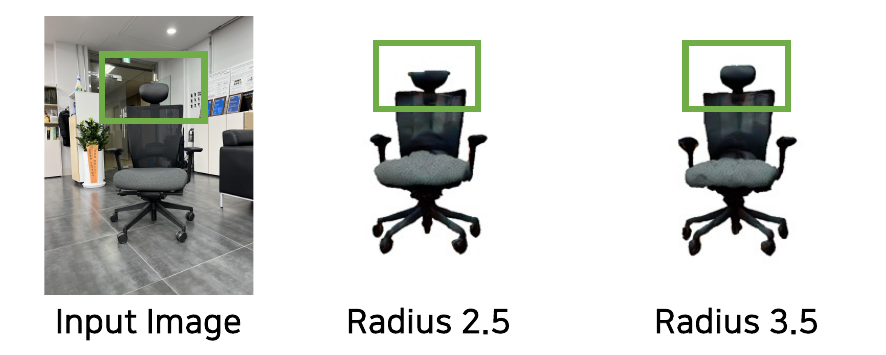}
    \caption{\textbf{The necessity of learnable virtual camera.} 
    Using an inappropriate radius in the virtual camera space can lead to issues such as exceeding the camera space boundaries, as seen in the green box, or causing degradation of details.
    }
  \label{fig:supp_radius}
\end{figure}
